# Supplementary material for: General Slit Stochastic L\"owner Evolution and Conformal Field Theory
Source: arXiv:1510.04123 source file (2026-11-22)
Supplement: Supplementary file 1 [file appendixA.tex]

\chapter{Some appendix}
